# Supplementary material for: Algorithms with Logarithmic or Sublinear Regret for Constrained Contextual Bandits
Source: arXiv:1504.06937 source file (2015-10-19)
Supplement: Supplementary file 1 [file appendix_backup.tex]

%\newpage
%APPENDICES are optional
%\balancecolumns
\appendices
%Appendix A

%%%%%%%%%%
\section{Proof of Proposition 1}\label{app:proof_opt_threshold_struct}
%%%%%%%%%%
Define the dynamic programming (DP) value function $V_{\tau}(b)$ as the maximum expected total rewards when the remaining time is $\tau$ and remaining budget is $b$. This value function can be expressed in a recursive manner:

When $\tau = 0$, $V_0(b) = 0$ for all $b \in \mathbb{N}$.

When $\tau > 0$, the policy makes decision based on the context $Z_{T-\tau}$ and remaining budget $b$. When $b > 0$, the policy can choose to {\it pull} the optimal arm for $Z_{T-\tau}$ ($\nu = 1$) or {\it wait} for the next context ($\nu = 0$). When the  budget is run out, i.e., $b= 0$, the policy cannot pull any arms ($\nu = 0$).   According to the Bellman equation, we can express $V_{\tau}(b)$ with respect to the value function in the next time-slot:
\begin{eqnarray}
V_{\tau}(b) = \mathbb{E}_{Z_{T - \tau}}\big\{\max_{\nu \in \{0, 1\land b\}} [\nu u_{Z_{T - \tau}}^* + V_{\tau-1}(b - \nu)] \big\},
\end{eqnarray}
where $1 \land b = \min\{1,b\}$.

When $b > 0$, $\tau > 0$, and $Z_{T- \tau} = j$, an optimal policy should choose an action $\nu \in \{0, 1\}$ that maximizes $\nu u_{Z_{T - \tau}}^* + V_{\tau-1}(b - \nu)$, i.e.,
\begin{eqnarray}
V_{\tau -1}(b) \underset{\nu = 1}{\overset{\nu = 0}{\gtrless}} u_j^* + V_{\tau-1}(b - 1).
\end{eqnarray}
This decision criterion can be rewritten as
\begin{eqnarray}
V_{\tau-1}(b) - V_{\tau-1}(b - 1)\underset{\nu = 1}{\overset{\nu = 0}{\gtrless}} u_j^*.
\end{eqnarray}
This implies that if $\nu = 1$ for context $j$, then $\nu = 1$ for all $j' > j$.

On the other hand, for given $j$, if $V_{\tau-1}(b+1) - V_{\tau-1}(b) \leq V_{\tau-1}(b) - V_{\tau-1}(b - 1)$, i.e., $V_{\tau-1}(b+1) + V_{\tau-1}(b - 1) \leq 2V_{\tau-1}(b)$, then  $\nu = 1$ for remaining budget $b$ implies $\nu = 1$ for all $b' > b$. Namely, the concavity of the value function on $\mathbb{N}$ is a sufficient condition of the threshold structure. We can show the concavity of $V_{\tau}(b)$ by induction to $\tau$.

When $\tau = 0$,
$V_0(b)$ is concave on $\mathbb{N}$ since $V_0 (b) = 0$ for all $b \in \mathbb{N}$. For $\tau > 0$, assume $V_{\tau-1}(b)$ is a concave function on $\mathbb{N}$. Let $V_{\tau,j}(b)$ be the value function conditioned on $Z_{T-\tau} = j$, i.e.,
\begin{eqnarray}
V_{\tau,j}(b) &=& \max_{\nu \in \{0, 1\land b\}} [\nu u_j^* + V_{\tau-1}(b - \nu)].
\end{eqnarray}
We note that when $b \geq 1$, $V_{\tau,j}(b) = \max_{\nu \in \{0, 1\}} [\nu u_j^* + V_{\tau-1}(b - \nu)]$ is concave since the maximization operation preserves concavity. To extend the concavity to the entire set of $\mathbb{N}$, it suffices to show that
\begin{eqnarray}\label{eq:grad_1}
V_{\tau,j}(0) + V_{\tau,j}(2) \leq 2V_{\tau,j}(1).
\end{eqnarray}
Note that
\begin{eqnarray}
V_{\tau,j}(0) &=& 0, \nonumber \\
V_{\tau,j}(2) &=& \max\{V_{\tau-1}(2), u_j^* + V_{\tau-1}(1)\}, \nonumber\\
2V_{\tau,j}(1) & = & \max\{2V_{\tau-1}(1), 2u_j^*  \} \nonumber.
\end{eqnarray}
Further, $u_j^* + V_{\tau-1}(1) \leq \max\{2V_{\tau-1}(1), 2u_j^*  \}$, and $V_{\tau-1}(2) = V_{\tau-1}(2) + V_{\tau-1}(0)\leq 2V_{\tau-1}(1)$ (because the concavity of $V_{\tau-1}(b)$ on $\mathbb{N}$). Thus, inequality~\eqref{eq:grad_1} holds and $V_{\tau,j}(b)$ is concave on $\mathbb{N}$, and $V_{\tau}(b) = \mathbb{E}_{Z_{T-\tau}}V_{\tau,Z_{T-\tau}}(b)$ is concave on  $\mathbb{N}$ because the expectation operation preserves concavity.

Consequently, $V_{\tau}(b)$ is concave on $\mathbb{N}$ for all $0 \leq \tau \leq T$, and the threshold policy is optimal.

%%%%%%%%%%
\section{Proof of Proposition 3}\label{app:proof_opt_twophase_policy}
%%%%%%%%%%

We first compare the exploit-phase with the original system. Note that $V_T(B)$ is the maximum expected total reward in the original problem and  $V_{T-\epsilon \log T}(B - \epsilon \log T)$ is the maximum expected total reward in the exploit-phase under the Two-Phase policy. When $T$ is sufficiently large such that $B - \epsilon \log T > 0$, by the Bellman's equality, we have
\begin{eqnarray}
V_{T}(B) &=& \mathbb{E}_{Z_{T}}\big\{\max_{\nu \in \{0, 1\}} [\nu u_{Z_{T}}^* + V_{T-1}(B - 1)] \big\}\nonumber \\
&\leq& u^* + V_{T-1}(B-1) \nonumber \\
&& \ldots \nonumber \\
&\leq & (\epsilon \log T)u^* + V_{T-\epsilon \log T}(B - \epsilon \log T).
\end{eqnarray}

Next, we show that based on the statistics learned from the explore-phase, the agent takes exactly the optimal actions in each time-slot with high probability in the exploit-phase.

Specifically, let $N_j$ be the number of occurrences of context $j$ in the explore phase, i.e., $N_j = \sum_{t = 0}^{T_1 -1} {\textbf{1}}(Z_t = j)$, and $N_{j,k}$ be the number of pullings for arm $k$ under context $j$. Then, for $0 < \delta_1 < \underline{\pi}$, by Chernoff-Hoeffding bound, we have
\begin{eqnarray}
\mathbb{P}\{N_j \geq (\pi_j - \delta_1) T_1\} \geq 1 - e^{-2 \delta_1^2 T_1} = 1 - T^{-2\epsilon \delta_1^2},
\end{eqnarray}
and
\begin{eqnarray}
\mathbb{P}\{N_{j,k} \geq \frac{(\pi_j - \delta_1) T_1}{K}\} \geq 1 - T^{-2\epsilon \delta_1^2}.
\end{eqnarray}
Moreover, according to Chernoff-Hoeffding bound, we have $\delta_2 > 0$, for each $j$ and $k$, and,
\begin{eqnarray}
\mathbb{P}\{\hat{u}_j(k) \geq u_j(k) + \delta_2\big|N_{j,k}\} \leq e^{-2\delta_2^2 N_{j,k}}, ~~j = 1, 2, \ldots, J; k = 1,2,\ldots, K.
\end{eqnarray}
Thus,
\begin{eqnarray}\label{eq:each_upper}
\mathbb{P}\{\hat{u}_j(k) \geq u_j(k) + \delta_2\big\} &\leq&  e^{-2\delta_2^2 (\pi_j - \delta_1) T_1/K} + T^{-2\epsilon \delta_1^2} \nonumber \\
&\leq& T^{-2\epsilon \delta_2^2 (\pi_j - \delta_1) /K} + T^{-2\epsilon \delta_1^2} \nonumber \\
&\leq& 2 T^{-2 \epsilon\zeta(\delta_1, \delta_2)},
\end{eqnarray}
where $\zeta(\delta_1, \delta_2) = \min\{\delta_2^2 (\pi_j - \delta_1) /K, \delta_1^2\}$.

Similarly,
\begin{eqnarray}\label{eq:each_lower}
\mathbb{P}\{\hat{u}_j(k) \leq u_j(k) - \delta_2\} \leq 2 T^{-2 \epsilon\zeta(\delta_1, \delta_2)}.
\end{eqnarray}


On the other hand, during the exploit-phase, the sequence of actions taken by the two-phase policy dismatches the optimal solution (denoted as $\mathcal{E}_{\rm error}$) only when at least one of the following event is true: (\red{we assume the optimal arm for each context is unique, and the ``better'' context is unique}):
\begin{eqnarray}
&&\mathcal{E}_{j} = \{\exists k \neq k_j^*,~\hat{u}_j(k) \geq \hat{u}_j(k_j^*)\}, j = 1,2,\ldots, J,\label{eq:viol_each} \\
&&\mathcal{E}^* = \{\exists j \neq j^*, \hat{u}_j^* \geq \hat{u}_{j^*}^*\}\label{eq:viol_opt}.
\end{eqnarray}
With respect to $\mathcal{E}_{j}$,
\begin{eqnarray}
\mathbb{P}(\mathcal{E}_{j}) &\leq& \sum_{k\neq k_j^*}\mathbb{P} \{\hat{u}_j(k) \geq \hat{u}_j(k_j^*)\}\nonumber \\
&\leq & \sum_{k\neq k_j^*}\big[\mathbb{P} \{\hat{u}_j(k) \geq u_j(k) + \frac{\Delta_{j,k}}{2}\} + \mathbb{P} \{\hat{u}_j(k_j^*) \leq {u}_j(k_j^*) - \frac{\Delta_{j,k}}{2}\}\big] \nonumber \\
& \leq & 2 \sum_{k\neq k_j^*} T^{-2 \epsilon \zeta(\delta_1, \frac{\Delta_{j,k}}{2})}\leq 2(K-1)T^{-2 \epsilon \zeta_{j, \min}},
\end{eqnarray}
where $\Delta_{j,k} = u_j^* - u_j(k)$, and $\zeta_{j, \min} = \min_{k \neq k_j^*}\zeta(\delta_1, \frac{\Delta_{j,k}}{2})$.

With respect to $\mathcal{E}^*$,
\begin{eqnarray}
\mathbb{P}(\mathcal{E}^*) &\leq& \sum_{j\neq j^*}\mathbb{P} \{\hat{u}_j^* \geq \hat{u}_{j^*}^*\}\nonumber \\
&\leq & \sum_{j\neq j^*} \sum_{k=1}^K \mathbb{P} \{\hat{u}_j(k) \geq \hat{u}_{j^*}(k_{j^*}^*)\}\nonumber\nonumber \\
&\leq & \sum_{j\neq j^*} \sum_{k=1}^K\big[ \mathbb{P} \{\hat{u}_j(k) \geq u_j(k) + \frac{\Delta^*_{j,k}}{2} \} + \mathbb{P}\{ \hat{u}_{j^*}(k_{j^*}^*) \leq {u}_{j^*}(k_{j^*}^*) - \frac{\Delta^*_{j,k}}{2}\} \big]\nonumber \\
&\leq & 2\sum_{j\neq j^*} \sum_{k=1}^K T^{-2 \epsilon \zeta(\delta_1,\sum_{j\neq j^*} \sum_{k=1}^K )} \leq 2(J-1)K T^{-2\epsilon \zeta^*_{\min}},
\end{eqnarray}
where $\Delta^*_{j,k} = {u}_{j^*}(k_{j^*}^*) - u_j(k)$ and $\zeta^*_{\min} = \min_{j\neq j^*, k}\zeta(\delta_1,\frac{\Delta^*_{j,k}}{2})$.

Therefore, the probability that wrong actions are taken in the exploit-phase satisfies
\begin{eqnarray}
\mathbb{P}(\mathcal{E}_{\rm error}) &\leq& \sum_{j=1}^J \mathbb{P}(\mathcal{E}_j) + \mathbb{P}(\mathcal{E}^*)\nonumber \\
&\leq& \sum_{j=1}^J 2(K-1)T^{-2 \epsilon \zeta_{j, \min}} + 2(J-1)K T^{-2\epsilon \zeta^*_{\min}}.
\end{eqnarray}
Choosing a sufficiently large $\epsilon$ such that $\epsilon \zeta_{j, \min} \geq 1$ for all $j$ and $\epsilon \zeta^*_{\min}\geq 1$, we have
\begin{eqnarray}
\mathbb{P}(\mathcal{E}_{\rm error}) &\leq& 2 J(K-1)T^{-2} + 2 (J-1)KT^{-2} \leq 4JK T^{-2}.
\end{eqnarray}

Consequently, the worse-case regret is upper bounded by
\begin{eqnarray}
\bar{R}(B, T; \Gamma_{\rm 2-phase}) &\leq& V_{T}(B) - V_{T-\epsilon \log T}(B - \epsilon \log T) + \mathbb{P}(\mathcal{E}_{\rm error})(T-\epsilon\log T)u^* \nonumber \\
&\leq& (\epsilon \log T)u^* + u^*/T = O(\log T).
\end{eqnarray} 
